# Supplementary material for: Stream Runtime Monitoring on UAS
Source: arXiv:1804.04487 source file (2018-03-29)
Supplement: Supplementary file 1 [file appendix.tex]

\appendix
\textcolor{red}{kannst du ja frei rauskuerzen was du brauchst}\\
\begin{definition}{\emph{Syntactic Extensions}}\\ 
A \lola~Specification represents an equation system over typed \emph{stream variables} of the form:
\vspace{-2mm}
\begin{align*}	
    \textbf{input}&\ T_1\ t_1\\ \vspace{-5mm}
    \dots   \\\vspace{-5mm}
    \textbf{input}&\ T_m\ t_m\\\vspace{-5mm}
	\textbf{output}&\ T_{m+1}\ s_1   :=  e_1(t_1,\dots,t_m, s_1, \dots s_n)&  \\ \vspace{-5mm}
	\dots   \\\vspace{-5mm}
	\textbf{output}&\ T_{m+n}\ s_n   :=  e_n(t_1,\dots,t_m, s_1, \dots s_n) &
\end{align*} 
The \emph{independent} stream variables $t_1,\dots,t_m$ refer to input streams, and the stream variables $s_1,\dots,s_n$ refer to output streams.
The independent stream variable $t_1,\dots,t_m$ are typed $T_1,\dots,T_m$ and the dependent stream variable $s_1,\dots,s_n$ are typed $T_{m+1},\dots,T_{m+n}$.
The values of the output streams $s_i$ are given by evaluating the respective stream expression $e_i(t_1,\dots,t_m, s_1, \dots s_n)$, where $1 \leq i \leq n$ and $s_i$ and $e_i$ have the same type.
A stream expression $e(t_1,\dots,t_m, s_1, \dots s_n)$ is defined recursively as follows:
\begin{itemize}
\item Let $a$ be keyword of type $T$ (e.g.~\texttt{position} or \texttt{int\_min}, \texttt{int\_max} representing the maximal ints), then $e\widehat{=}a$ is an atomic stream expression of type T.
%\item Let $e_c$ be a stream expression of type $T'$, $c_1,\dots,c_l$ be constants of type $T'$, and $e_1,\dots,e_l, e_{l+1}$ be stream expressions of type $T$, then\\ $e= switch\ e_c\ \{\ case\ c_1\ \{e_1\}\ \dots\ case\ c_l\ \{e_l\}\ default \{e_{l+1}\}\ \}$ is a stream expression of type $T$. Furhter, if $e_c$ is a stream variable and flagged monotonically increasing or decreasing\footnote{\texttt{monoton\_inc} $e_c$ and \texttt{monoton\_dec} $e_c$ declare that the stream values are increasing or decreasing respectively.} then $c_1,\dots,c_l$ have to be ordered increasingly or decreasingly, respectively.
\item Let $e'$ be a stream expression of type $T$, $d$ a constant of type $T$, $i$ an int, and $ft$ an \emph{optional} positive int by default $0$, then $e\widehat{=}e'[i,d,ft]$ is a stream expression of type $T$. 
\item Let $e'$ be a stream expression of type $T$, $d$ a constant of type $T$, and $i$ an positive int, then $e\widehat{=}e'\#[i,d]$ is a stream expression of type $T$. 
\end{itemize} 
Common abbreviations:
\vspace{-3mm}
\begin{itemize}
\item[$\bullet$]\texttt{const T s := a $\widehat{=}$ output T s := a}
\item[$\bullet$]\texttt{ite($e_1$,$e_2$,$e_3$) $\widehat{=}$ if $e_1$\{$e_a$\}else\{$e_b$\}}
\item[$\bullet$]\texttt{if $e_1$\{$e_a$\}elif $e_2$\{$e_b$\}else\{$e_c$\} $\widehat{=}$ if $e_1$\{$e_a$\}else\{if$e_2$\{$e_b$\}else\{$e_c$\}\}}
\item[$\bullet$] \texttt{plus($e_a,e_b$) $\widehat{=}$ $e_a + e_b$}, the same holds for other common functions. The order of precedence is as expected.
\item[$\bullet$]\texttt{if $e_a=c_1$\{$e_1$\}elif $e_a=c_2$\{$e_2$\} $\dots$ elif $e_a=c_n$\{$e_n$\}else\{$e_d$\} $\widehat{=}$ \newline switch $e_a$\{ case $c_1$\{$e_1$\} case $c_2$\{$e_2$\} $\dots$ case $c_n$\{$e_n$\} default\{$e_d$\}\}}
\end{itemize}
\end{definition}

%%%%%%%%%%%%%%%%%%%%%%%%%%%%
%%%%%%%%%%%%%%%%%%%%%%%%%%%%
%  Semantics
%%%%%%%%%%%%%%%%%%%%%%%%%%%%
%%%%%%%%%%%%%%%%%%%%%%%%%%%%
\begin{definition}{\emph{Semantics Extensions}}\\
Let $\Phi$ be a specification with independent stream variables $t_1,\dots,t_m$ and dependent stream variable $s_1,\dots,s_n$.
The evaluation of the stream variables such that the underlying equation system is satisfied defines the semantics of a \lola~specification.
Given an input trace $\tau \widehat{=} \langle\tau_1,\dots,\tau_m\rangle$ of length $N+1$ for each independent stream $t_1,\dots,t_m$ , the evaluation over the trace is defined as a stream of $N+1$ tuples $\langle\sigma_1,\dots,\sigma_n\rangle$ for each dependent stream variable $s_i$, such that for all $0 \leq j \leq N$ and $1 \leq i \leq n$, the following equations are satisfied:
%\begin{align*}
$\sigma_i(j) = val(e_i)(j)$
%\end{align*}
Such an equation satisfying evaluation is called an \emph{evaluation model}.
The function $val$ is inductively defined as follows:\\
\emph{Base case extensions:}\qquad\qquad $val(position)(j) = j$\qquad \footnote{The respective maximal value for \texttt{int\_min, int\_max, double\_min, double\_max}.}\\
%\begin{itemize}
%\item $val(position)(j) = j$\qquad \footnote{The respective maximal value for \texttt{int\_min, %int\_max, double\_min, double\_max}.}
%\end{itemize}
\emph{Inductive case extensions:}%, where $e_1,\dots,e_k$ are sub-expressions:}
\vspace{-3mm}
\begin{itemize}
%\item $eval(switch\ e_k\ \{\ case\ c_1\ \{e_1\}\ \dots\ case\ c_{k-2}\ \{e_{k-2}\}\ default \{e_{k-1}\}\ \})(j)=
%\begin{cases}
%	\begin{cases}
%	eval(e_1)(j) &, \text{if}\ eval(e_k) = c_1\\
%	...&\\
%	eval(e_{k-2})(j) &, \text{if}\ eval(e_{k}) = c_{k-2}\\
%	eval(e_{k-1})(j) &, otherwise\\
%	\end{cases} &, \text{if}\ state\ \text{is}\ undef\\
%	\begin{cases}
%	eval(e_{state})(j);\ state := state &, \text{if}\ eval(e_k) = c_{state}\\
%	...&\\
%	eval(e_{k-2})(j);\ state := k-2 &, \text{if}\ eval(e_{k}) = c_{k-2}\\
%	eval(e_{k-1})(j);\ state := k-1 &, otherwise\\
%	\end{cases}  &, \text{otherwise.}
%\end{cases}$\\
%, where $c_1,\dots,c_l$ are constants, $state$ is an auxiliary variable initialized to \emph{undef} if $e_k$ is neither a monotonically increasing nor monotonically decreasing stream variable, if it is a monotonically increasing stream variable then it is initialized to the first case block, otherwise to the default block.
\item $eval(e[p,d,ft])(j)=
\begin{cases}
	eval(e)(j+p) &, \text{if}\ j\%(ft+1)=0\ \text{and}\ 0 \leq p \leq N\\
	eval(d)(j)   &, \text{if}\ j\%(ft+1)=0\ \text{and}\ p > N\\
	eval(e)(j-1) &, otherwise
\end{cases}$
\item $eval(e\#[p,d])(j) =
	\begin{cases}
		eval(e)(p) &,\ \text{if}\ 0 \leq p \leq N\\
		eval(d)(j) &, \text{otherwise}
	\end{cases}$
\end{itemize}
\end{definition}
